# Supplementary material for: Electron-Beam Driven Relaxation Oscillations in Ferroelectric Nanodisks
Source: arXiv:1505.02327 source file (2015-05-09)
Supplement: Supplementary file 1 [file faceting-supp.pdf]

# Supplementary Material - Electron-Beam Driven Relaxation Oscillations in Ferroelectric Nanodisks

Nathaniel Ng and Rajeev Ahluwalia
*Institute of High Performance Computing, Singapore 138632, Singapore*

Ashok Kumar
*National Physical Laboratory (CSIR), India*

David J. Srolovitz
*Departments of Materials Science and Engineering, Mechanical Engineering and Applied Mechanics, University of Pennsylvania, Philadelphia, Pennsylvania 19104, USA*

Premala Chandra
*Department of Physics and Astronomy, Rutgers University*

James F. Scott
*Department of Physics, Cavendish Laboratory, J. J. Thompson Avenue, Cambridge CB3 0HE, United Kingdom and St. Andrews, United Kingdom*

(Dated: May 10, 2015)

## MODEL

### Overview

A phase field model with both elastic and electrostatic interactions is employed, based on earlier works [1–3] but has been adapted to incorporate the circular geometry, by use of a shape function, $c = c(\mathbf{r})$, where:

$$c = \begin{cases} 0, & \text{outside the perimeter of the circle} \\ 1, & \text{inside the perimeter of the circle} \end{cases} \tag{1}$$

The polarizations are set to zero outside the perimeter of the circle.

The electron beam effects enter the model through a non-zero space charge in the Maxwell equation [4].

### Total Free Energy

The total free energy, $F_T$ is given by:

$$F_T = \int d\mathbf{r}\,(f_L + f_G + f_{\text{elastic}}) \tag{2}$$

where $f_L$ is the local free energy, $f_G$ is the gradient energy, and $f_{\text{elastic}}$ is the elastic free energy. The definitions of each term are given as follows.

### Local Free Energy

The 2D, 8th order polynomial expansion for $f_L(\mathbf{P}), \mathbf{P} = (P_x, P_y)^T$ is [5]:

$$\begin{aligned} f_L(\mathbf{P}) = &\alpha_1 \left(P_x^2 + P_y^2\right) + \alpha_{11}\left(P_x^4 + P_y^4\right) \\ &+ \alpha_{12} P_x^2 P_y^2 + \alpha_{111}\left(P_x^6 + P_y^6\right) \\ &+ \alpha_{112}\left(P_x^4 P_y^2 + P_x^2 P_y^4\right) \\ &+ \alpha_{1111}\left(P_x^8 + P_y^8\right) \\ &+ \alpha_{1112}\left(P_x^6 P_y^2 + P_y^6 P_x^2\right) + \alpha_{1122}\left(P_x^4 P_y^4\right) \end{aligned} \tag{3}$$

where $\alpha_1, \alpha_{11}, \alpha_{12}, \alpha_{111}, \alpha_{112}, \alpha_{1111}, \alpha_{1112}, \alpha_{1122}$ are constants for PZT obtained from Haun et al [6].

### Gradient Energy

The gradient energy is:

$$\begin{aligned} f_G(\nabla \mathbf{P}) &= \frac{1}{2} c\kappa \left|\nabla \mathbf{P}\right|^2 \\ &= \frac{1}{2} c\kappa \left(\left|P_{x,x}\right|^2 + \left|P_{y,y}\right|^2\right) \end{aligned} \tag{4}$$

Here, $\kappa$ is a coefficient for the isotropic gradient energy, and we have multiplied it by $c(\mathbf{r})$ so that it vanishes outside the perimeter.

### Elasticity

The elastic energy is given by:

$$\begin{aligned} f_{\text{elastic}} = &\ \tfrac{1}{2} C_{11}\left(e_{xx}^2 + e_{yy}^2\right) \\ &+ C_{12}\left(e_{xx} e_{yy}\right) + \tfrac{1}{2} C_{44}\left(e_{xy}^2\right) \end{aligned} \tag{5}$$

where $e_{ij}$ is the elastic strain given by:

$$e_{ij} = \varepsilon_{ij} - \varepsilon^0_{ij} \tag{6}$$

where we define the transformational strains, $\varepsilon^0_{ij}$ as:

$$\begin{aligned} \varepsilon^0_{xx} &= Q_{11}P_x^2 + Q_{12}P_y^2 \\ \varepsilon^0_{yy} &= Q_{12}P_x^2 + Q_{11}P_y^2 \\ \varepsilon^0_{xy} &= Q_{44}P_xP_y \end{aligned} \tag{7}$$

The strains are calculated from the displacement fields as:

$$\begin{aligned} \varepsilon_{yy} &= u_{y,y} \\ \varepsilon_{xx} &= u_{x,x} - \tfrac{C_{12}}{C_{11}}\left(\varepsilon_{yy} - \varepsilon^0_{yy}\right) \\ \varepsilon_{xy} &= \tfrac{1}{2}\left(u_{x,y} + u_{y,x}\right) \end{aligned} \tag{8}$$

The stress fields are obtained from equations 8 and 9 as:

$$\begin{aligned} \sigma_{xx} &= c\left(\mathbf{r}\right)\left[C_{11}\left(\varepsilon_{xx} - \varepsilon^0_{xx}\right) + C_{12}\left(\varepsilon_{yy} - \varepsilon^0_{yy}\right)\right] \\ \sigma_{yy} &= c\left(\mathbf{r}\right)\left[C_{12}\left(\varepsilon_{xx} - \varepsilon^0_{xx}\right) + C_{11}\left(\varepsilon_{yy} - \varepsilon^0_{yy}\right)\right] \quad (9) \\ \sigma_{xy} &= c\left(\mathbf{r}\right)C_{44}\left(\varepsilon_{xy} - \varepsilon^0_{xy}\right) \quad (10) \end{aligned}$$

### Kinetics for the Polarizations

The polarizations evolve according to [7, 8] (with evolution outside the perimeter of the circle ignored):

$$\frac{1}{\Gamma}\frac{\partial \mathbf{P}}{\partial t} = \begin{cases} \nabla\cdot\left(\frac{\partial F_T}{\partial \nabla \mathbf{P}}\right) - \frac{\partial F_T}{\partial \mathbf{P}} - \nabla\phi, & \text{if } c = 1 \\ 0, & \text{if } c = 0 \end{cases} \tag{11}$$

where $\Gamma$ is a kinetic coefficient indicative of the domain wall mobility and $\phi$ is the electrostatic potential obtained from the Maxwell equation, as described below.

### Electrostatics

The electrostatic potential, $\phi\left(\mathbf{r}\right)$, is obtained by solving Maxwell's equation for a given polarization distribution, $\mathbf{P}\left(\mathbf{r}\right)$, and charge distribution, $\rho = \rho\left(\mathbf{r}\right) = -c\left(\mathbf{r}\right)qN_e$ and $\chi_b = \chi_b\left(\mathbf{r}\right)$ is the background dielectric constant:

$$\nabla\cdot\left[-\epsilon_0\left(1+\chi_b\right)\nabla\phi + \mathbf{P}\right] = \rho \tag{12}$$

In the vacuum (i.e. $c\left(\mathbf{r}\right) = 0$), $\mathbf{P} = \mathbf{0}, \chi_b = 0$, and $\rho = 0$; inside the solid, $\mathbf{P}$ is obtained from the phase field equation, $\chi_b = 9$, and $\rho = -qN_e$.

### Elastodynamics

In equation 11, we also need to solve for the displacement / elastic fields. The elastodynamic equation is used to drive the system to mechanical equilibrium:

$$\begin{aligned} \tilde{\rho}\frac{\partial^2 u_x}{\partial t^2} &= \sigma_{xx,x} + \sigma_{xy,y} + \eta\nabla^2\dot{u}_x \\ \tilde{\rho}\frac{\partial^2 u_y}{\partial t^2} &= \sigma_{xy,x} + \sigma_{yy,y} + \eta\nabla^2\dot{u}_y \end{aligned} \tag{13}$$

where $\tilde{\rho}$ is the density, and $\eta$ is a damping constant.

At the limit $t \to \infty$, $\ddot{u} \to 0$ and $\dot{u} \to 0$, so equation 14 becomes:

$$\begin{aligned} 0 &= \sigma_{xx,x} + \sigma_{xy,y} \\ 0 &= \sigma_{xy,x} + \sigma_{yy,y} \end{aligned} \tag{14}$$

which is the mechanical equilibrium equation.

## SIMULATION

### Discretization

Variables such as $\mathbf{P}, \mathbf{E}, \phi, \rho$ are assumed to be spatially varying (i.e. $\mathbf{P} = \mathbf{P}\left(\mathbf{r}\right)$, etc. where $\mathbf{r} = \left(x, y\right)^T$). All spatially-varying variables are discretized onto a 2D grid of size $n_i \times n_j$. The polarizations are evolved using Euler time stepping in a finite difference method implementation with second order symmetric stencils.


[1] R. Ahluwalia, N. Ng, and D. J. Srolovitz, "Surface morphology effects on polarization switching in nanoscale ferroelectrics," *Nanotechnology*, vol. 20, no. 44, p. 445709, 2009.

[2] N. Ng, R. Ahluwalia, and D. J. Srolovitz, "Domain patterns in free-standing nanoferroelectrics," *Acta Materialia*, vol. 60, p. 3632–3642, May 2012.

[3] R. Ahluwalia, N. Ng, A. Schilling, R. G. P. McQuaid, D. M. Evans, J. M. Gregg, D. J. Srolovitz, and J. F. Scott, "Manipulating ferroelectric domains in nanostructures under electron beams," *Physical Review Letters*, vol. 111, Oct 2013.

[4] N. Ng, R. Ahluwalia, and D. J. Srolovitz, "Depletion-layer-induced size effects in ferroelectric thin films: A ginzburg-landau model study," *Physical Review B*, vol. 86, no. 9, p. 094104, 2012.

[5] Y. L. Li, L. E. Cross, and L. Q. Chen, "A phenomenological thermodynamic potential for batio$_3$ single crystals," *Journal of Applied Physics*, vol. 98, p. 064101, 2005.

[6] M. J. Haun, Z. Q. Zhuang, E. Furman, S. J. Jang, and L. E. Cross, "Thermodynamic theory of the lead zirconate-titanate solid solution system, part III: curie constant and sixth-order polarization interaction dielectric stiffness coefficients," *Ferroelectrics*, vol. 99, no. 1, pp. 45–54, 1989.

[7] Y. Xiao, V. B. Shenoy, and K. Bhattacharya, “Depletion layers and domain walls in semiconducting ferroelectric thin films,” *Physical Review Letters*, vol. 95, p. 247603, 2005.

[8] P. Suryanarayana and K. Bhattacharya, “Evolution of polarization and space charges in semiconducting ferroelectrics,” *Journal of Applied Physics*, vol. 111, p. 034109, 2012.
